# Supplementary material for: Amplitude analysis of the $D_s^+ \to \pi^- \pi^+ \pi^+$ decay
Source: arXiv:2209.09840 source file (2023-10-17)
Supplement: Supplementary file 1 [file appendix.tex]

% ===============================================================================
% Purpose: appendix to the standard template: standard symbol alises from Ulrik
% Author: Tomasz Skwarnicki
% Created on: 2009-09-24
% ===============================================================================

%{\noindent\normalfont\bfseries\Large Appendices}
\section*{Appendix}

%\appendix

\section*{Parameterisation of the $P$ and $D$-waves}

 The relativistic Breit-Wigner function is defined as
\begin{eqnarray}
T_{R}(m)=\frac{1}{m_{0}^{2}-m^2-i m_{0} \Gamma(m)},
\end{eqnarray}
where $m$ is the $\pim\pip$ ~invariant mass, $m_0$ and $\Gamma(m)$ are the  resonance mass and mass-dependent width, respectively. The mass-dependent width is expressed as
\begin{eqnarray}
\Gamma\left(m\right)=\Gamma_{0}\left(\frac{p}{p_{0}}\right)^{2 L+1} \frac{m_{0}}{m} \frac{F_{R}^{2}(z)}{F_{R}^{2}\left(z_{0}\right)}.
\end{eqnarray}
The symbol $\Gamma_0$ denotes the nominal width of the resonance, $p$ is the decay momentum, $p_0$ is its value at $m=m_0$, and $z_0$ is calculated when $p=p_0$. The values $m_0$ and $\Gamma_0$ for all resonances are fixed in the fit. Finally, $F_R(z)$ is the Blatt-Weisskopf barrier factor listed in Table \ref{table:blatt}.

The Gounaris-Sakurai function is a modification of the RBW lineshape,
\begin{equation}
T_{GS}(m) =  \frac{1+\Gamma_0d/m_0}{(m_0^2 - m^2) + f(m) - i m_0 \Gamma(m)}, 
\end{equation}
where
 \begin{equation}
\begin{split}
f(m) &= \Gamma_0 \,\frac{m_0^2}{p_0^3}\,\left[\; p^2 \left(h(m)-h(m_0)\right) +
       \left(\,m_0^2-m^2\,\right)\,p^2_0\,
       \frac{dh}{dm}\bigg|_{m_0}
       \;\right]. \\
    \end{split}
\end{equation}

The function $h(m)$ is given by
\begin{equation}
    h(m) = \frac{2}{\pi}\,\frac{p}{m}\,
       \ln\left(\frac{m+2p}{2m_\pi}\right)~, \\
\end{equation}
where $m_{\pi}$ is the pion mass and with 
\begin{equation}
\frac{dh}{dm}\bigg|_{m_0} =
h(m_0)\left[(8p_0^2)^{-1}-(2m_0^2)^{-1}\right] \,+\, (2\pi m_0^2)^{-1}~. \\
\end{equation}

The parameter $d=f(0)/(\Gamma_0 m_0)$ is given by
\begin{equation}
  d = \frac{3}{\pi}\frac{m_\pi^2}{p_0^2}
  \ln\left(\frac{m_0+2p_0}{2m_\pi}\right)
  + \frac{m_0}{2\pi\,p_0}
  - \frac{m_\pi^2 m_0}{\pi\,p_0^3}~.
\end{equation}

In the analysis of the Dalitz plot the normalised Blatt-Weisskopf barrier factors~\cite{book:BlattWeisskopf}, $F_D^L$ and $F_R^L$, are used for the vertices $D_s^+\to R \pi^+$ and $R\to \pi^-\pi^+$, respectively. The barrier factors are defined in terms of $z\equiv |\vec{p}|r$, where $\vec{p}$ is the momentum of the decay products, always calculated in the rest frame of the decaying particle. The normalisation factor is defined in terms of $z_0 \equiv|\vec{p_0}|r$, so that $F_D^L,F_R^L=1$ when $m=m_0$. The values of the parameter $r$ are fixed at $r=r_{D} = 5.0$ GeV$^{-1}$ for the transition $D_s \rightarrow R \pi^+$, ~and $r=r_{R} = 1.5$ GeV$^{-1}$ for the transition $R \rightarrow \pi^-\pi^+$.The formulae for the form factors are summarised in Table \ref{table:blatt}.

The Lorentz-invariant functions $\mathcal{M}_J$ are obtained from the covariant tensor formalism. In the decay $D\to R c$, $R\to ab$, the expressions read
\begin{equation}
\mathcal{M}_{1} = s_{bc} - s_{ab} + \left(\frac{1}{s_{ab}} (m_D^2 - m_c^2) (m_a^2 - m_b^2)\right),
\label{spin1}
\end{equation}
for spin-1 resonances, and

\begin{multline}
\mathcal{M}_{2}= \mathcal{M}_{1}^2 - \frac{1}{3}\left(s_{ab} - 2m_D^2 -m_c^2 + \frac{1}{s_{ab}}(m_D^2-m_b^2)^2\right)\times \\ \left(s_{ab} - 2m_a^2 - 2m_c^2 + \frac{1}{s_{ab}}(m_a^2-m_b^2)^2 \right),
\label{spin2}
\end{multline}
for spin-2 resonances.

\begin{table}[h!] 
    \caption{Spin-dependent Blatt-Weisskopf barrier factors. The normalization ensures that the barrier factors are equal to one at the resonance mass.}
	\begin{center}
		\begingroup
\setlength{\tabcolsep}{10pt} % Default value: 6pt

		\begin{tabular}{ c  c }
		Resonance spin & Form factor\\
		\hline
%			1 & $\sqrt{\frac{1+ z_0^2}{1 + z^2}}$  \\ 
%			2 & $\sqrt{\frac{z_0^4 + 3z_0^2 + 9}{z^4 + 3z^2 + 9}}$  \\
						1 & $(1 + z_0^2)^{1/2}\times(1 + z^2)^{-1/2}$  \\ 
			2 & $(z_0^4 + 3z_0^2 + 9)^{1/2}\times(z^4 + 3z^2 + 9)^{-1/2}$  \\
			\hline  
		\end{tabular}
	\endgroup
	\end{center}
	\label{table:blatt}
\end{table}
